# Supplementary material for: RTAMT -- Runtime Robustness Monitors with Application to CPS and Robotics
Source: arXiv:2501.18608 source file (2025-01-22)
Supplement: Supplementary file 1 [file appendix.tex]

\appendix
\section{Preliminaries}
\subsection{Target}
Target journals,
\begin{itemize}
    \item International Journal on Software Tools for Technology Transfer\\
        \url{https://www.springer.com/journal/10009/}\\
        \url{https://www.guide2research.com/journal/international-journal-on-software-tools-for-technology-transfer-2}
    \item ACM Transactions on Programming Languages and Systems (TOPLAS)\\
        \url{https://www.guide2research.com/journal/acm-transactions-on-programming-languages-and-systems}
\end{itemize}
Just in case, Sriram suggested as Plan B
\begin{itemize}
    \item Logical Methods in Computer Science (LMCS)\\
        \url{https://lmcs.episciences.org/}\\
    \item ACM Transactions on Embedded Computing Systems (TECS)\\
        \url{https://dl.acm.org/journal/tecs}
\end{itemize}

\subsection{Word correction}
\begin{itemize}
    \item satisfied, not satisfied$\leftrightarrow$
        $[$satisfied, violated$]$$\leftrightarrow$
        valid, invalid$\leftrightarrow$
        positive, negative
    \item Robustness v.s. Quantitative semantics. We may use Robustness mainly, Quantitative semantics should be an explanation and supplement of that like explain logic.
    \item user $\leftrightarrow$ designer $\leftrightarrow$ specification designer
    $\leftrightarrow$ $[$practitioner$]$
    \item use case $\leftrightarrow$ $[$use-case$]$
    \item frontend $\leftrightarrow$ $[$front-end$]$
    \item backend $\leftrightarrow$ $[$back-end$]$
    \item real time $\leftrightarrow$ $[$real-time$]$
    \item discrete time $\leftrightarrow$ $[$discrete-time$]$
    \item dense time $\leftrightarrow$ $[$dense-time$]$
    \item $[$runtime$]$ $\leftrightarrow$ run-time
    \item runtime $\leftrightarrow$ online\\
        runtime: in paragraph.\\
        online: only in code because of compatibility of offline.
    \item monitor $\leftrightarrow$ evaluator $\leftrightarrow$ specification\\
        monitor: should be general name of the entire tool in paragraph.\\
        evaluator: one of name of class in code.\\
        specification: name of integrated class in code.
    \item $[$monitors$]$ $\leftrightarrow$ monitoring
    \item future-operator $\leftrightarrow$ future-temporal-operator $\leftrightarrow$ $[$future temporal operator$]$
    \item $[$online monitors, offline monitors$]$
    \item past-operator $\leftrightarrow$ past-temporal-operator $\leftrightarrow$ $[$past temporal operator$]$
    \item $[$MATLAB$]$ $\leftrightarrow$ matlab $\leftrightarrow$ Matlab
    \item $[$middleware$]$ $\leftrightarrow$ middle-ware
    \item $[$real-world$]$ $\leftrightarrow$ real world
    \item $[$subsystem$]$ $\leftrightarrow$ sub-system
\end{itemize}

\subsection{Backups}

\begin{figure*}[t]
    \centering
    \begin{minipage}{0.46\hsize}
        \centering
        \includegraphics[width=\linewidth]{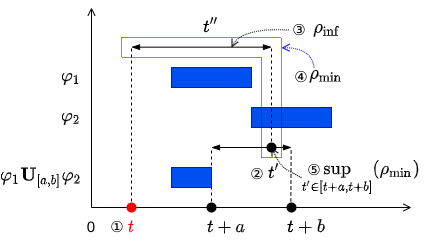}
        \label{fig:unitl}
        \subcaption{
        Until:\newline
        $\rob( \fun_1\,\until_{[a,b]}\,\fun_2, \signal, \timeElement)=\displaystyle\sup_{t' \in [\timeElement+a,\timeElement+b]} (\rho_{\min})$ \newline
        $\rob_{\min}=\min(\rob(\varphi_2, \signal, \timeElement'), \rob_{\inf})$\newline
        $\rob_{\inf}=\displaystyle\inf_{\timeElement'' \in [\timeElement,\timeElement')} \rob(\fun_1, \signal, \timeElement'')$
        }
    \end{minipage}
    \begin{minipage}{0.46\hsize}
        \includegraphics[width=\linewidth]{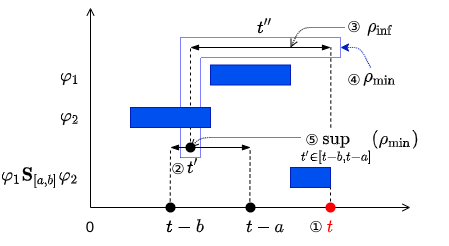}
        \subcaption{
        Since:\newline
        $\rob( \fun_1\,\since_{[a,b]}\,\fun_2, \signal, t)=\displaystyle\sup_{\timeElement' \in [\timeElement-b,\timeElement-a]}(\rho_{\min})$\newline
        $\rob_{\min}=\min(\rob(\varphi_2, \signal, \timeElement'), \rob_{\inf})$\newline
        $\rob_{\inf}=\displaystyle\inf_{\timeElement'' \in (\timeElement',\timeElement]} \rob(\fun_1, \signal, \timeElement'')$
        }
        \label{fig:since}
    \end{minipage}
    \caption{Semantics for $\until$ (Until) and $\since$ (Since) operators that are key formulas to enable $robustness$, and the difference: for simplicity, inputs $\fun_1$, $\fun_2$ are described as $\Bools$ even though they are $\Reals$. Let us elaborate on the $\until$ first.
    The intuitive semantics for the operator is seeking both $\fun_1$, $\fun_2$ with double loops with $t'$, $t''$ to evaluate all combinations of time steps on the inputs: 
    \circelNum{1} A formula is evaluated with respect to a time step $\timeElement$.
    \circelNum{2} $\timeElement'$ is an element in the interval $[\timeElement+a, \timeElement+b]$ from the given interval $[a,b]$.
    \circelNum{3} the infimum for  $\fun_1$ over $\timeElement$ and $\timeElement'$ is computed as $\rob_{\inf}$,
    \circelNum{4} minimum of the robustness at $\fun_2$ and $\rob_{inf}$ is evaluated at time $\timeElement'$.
    \circelNum{5} This process is repeated for every element $\timeElement' \in [\timeElement+a,\timeElement+b]$.
    The difference between $\until$ and $\since$ is 
    (a) $\timeElement'$ of $\sup$, $\timeElement''$ of $\inf$ in $\until$ seeks future data from current time $\timeElement$, 
    In contrast, 
    (b) $\timeElement'$, $\timeElement''$ in $\since$ seek past data from $\timeElement$.
    That enables $\since$ to evaluate in online fashion semantically since it does not need the future data.}
%    \label{fig:untilSince}
\end{figure*}

\newpage
\tableofcontents
